# Supplementary material for: Privacy-Preserving Public Information for Sequential Games
Source: arXiv:1402.4488 source file (2014-08-29)
Supplement: Supplementary file 1 [file future-appendix.tex]

\section{Future-dependent, Continuous Case}\label{section:future-appendix}
\begin{theorem}\label{thm:future-lb}
  There exist sequential resource-sharing games $g$, where each
  resource $r$'s value curve $\dvalo{r}$ is $\shallow{w}{n}$, such
  that in the future-dependent setting, $\comp_\greedy(\full, g) \geq
  2w$.
\end{theorem}
\begin{proof}
  Consider two players and two resources $r, r'$. Let $r$ have a value
  curve which is a step function, with $\val{0}{r} = w$, $\val{1}{r} =
  \frac{1}{2}$ and $\val{0}{r'} = w - \epsilon$. Suppose player one
  has access to both resources, the other having only resource $r$ as
  an option. Then, player one will choose $r$ according to greedy, and
  player two will always select $r$. The social welfare will be
  $SW(\greedy) = 1$, whereas $OPT$ is for player $1$ to take $r'$ and
  will have $SW(OPT) = 2w - \epsilon$. As $\epsilon \to 0$, this ratio
  approaches $2w$.
\end{proof}

Thus, as $w\to\infty$, the competitive ratio of the greedy strategy is
unbounded. Fortunately, the competitive ratio cannot be worse than
this, for fixed $w$, as we show in the theorem below.

\begin{theorem}\label{thm:full-dep}
  Suppose, for a sequential resource-sharing game $g$, each resource
  $r$'s value curve $v_r$ is $\shallow{w}{n}$. Then, in the in the
  future-dependent setting, $\comp_\greedy(\mech, g) =
  O(w\alpha\beta)$ for an $(\alpha, \beta)$-counter $\mech$.
\end{theorem}

\begin{proof}
  Let $PSW$ denote the perceived social welfare of a particular action
  set.  Consider a given player who chooses some set of resources
  according to the greedy strategy with respect to perfect
  information, with the impression that she should get value $V$ from
  her choices. That is, she chose $a_i$ such that

\[ a_i = \argmax_{a_i\in A_i}\sum_{r}\int_{\used{i}{r}}^{\used{i}{r} + \ract{i}{r}} \val{x}{r} dx \]

Then, we sum up the perceived utility all players have for their actions $a_i$:

\begin{equation}\label{eqn:shallow}
\begin{split}
 PSW(\greedy) = & \sum_{i\in [n]} \sum_{r}\int_{\used{i}{r}}^{\used{i}{r} + \ract{i}{r}} \val{x}{r} dx = \sum_{r}\int_{0}^{\used{n}{r} + \ract{n}{r}}\val{x}{r}dx\\
 \leq & w \left(\used{n}{r} + \ract{n}{r}\right)\val{\used{n}{r} + \ract{n}{r}}{r} = wSW(\greedy)
\end{split}
 \end{equation}
\noindent where the last inequality comes from our assumption about the value
curves all being $\shallow{w}{n}$. 

We now need to relate this quantity to $OPT$. Consider the game $g'$
where each player actually received her perceived payoff
$\sum_{r}\int_{\used{i}{r}}^{\used{i}{r} + \ract{i}{r}} \val{x}{r}dx$. It
is the case that $OPT_{g'}\geq OPT_g$. Moreover, players are choosing
their strategies greedily according to $g'$'s utility functions, so

\begin{align*}
  SW(\greedy, g) \geq \frac{1}{w}PSW(\greedy, g) =
  \frac{1}{w}SW(\greedy, g') \geq \frac{1}{4w} OPT_{g'} \geq
  \frac{1}{4w} OPT_g
\end{align*}

where the first inequality follows from (\ref{eqn:shallow}), the
second from the fact that $PSW(g, a) = SW(g', a)$ for all $a$, the
third from the fact that \greedy is $4$-competitive with $OPT$ for
$g'$ by Lemma~\ref{thm:greedy4}, and the final inequality follows from
$OPT_{g'}\geq OPT_g$.

The final part of the argument comes from the fact that the counters
are accurate within some quantity $\leq n$, so the perceived welfare
of greedy w.r.t the counter values and the perceived welfare of greedy
w.r.t. the true values are bounded by the appropriate quantity.
\end{proof}
